# Supplementary material for: Strong mixed-integer programming formulations for trained neural networks
Source: arXiv:1811.01988 source file (2020-01-21)
Supplement: Supplementary file 1 [file appendix-C.tex]

\section{Facet-defining proofs for Proposition~\ref{prop:max_big_m}} \label{app:max-big-m-facets}

The following lemma is useful for proving the result.

\begin{lemma} \label{lem:full-dimensionality}
    For each $k \in \llbracket d \rrbracket$, $D_{|k}$ is full-dimensional.
\end{lemma}
\proof{}
Given Assumption~\ref{ass:amphibious}, we are ensured that there exists some point $\hat{x} \in D$ such that $f^k(\hat{x}) > f^\ell(\hat{x})$ for each $\ell \neq k$. Moreover, as each function $\{f^\ell\}_{\ell=1}^d$ is linear, there exists some small $\epsilon > 0$ such that we may perturb $\hat{x}$ by this amount and continue in the interior of $D_{|k}$. More formally, there exists some $\epsilon > 0$ such that for each $x' \in B_\epsilon \defeq \Set{ x \in D | \: ||x-\hat{x}||_\infty < \epsilon}$, $f^k(x') > f^\ell(x')$ for each $\ell \neq k$. In other words, $B_\epsilon \subseteq D_{|k}$. From definition, $B_\epsilon$ has the same dimension as $D$, and as $B_\epsilon \subseteq D_{|k}$, the result follows.
\qed\endproof

\begin{proof}[Proposition~\ref{prop:max_big_m}]
We prove the result for \eqref{eqn:max_big_m-1}; the argument for \eqref{eqn:max_big_m-2} follows in the same manner, merely interchanging an $\arg\max$ for an $\arg\min$ below.

Note that, under Assumption~\ref{ass:amphibious}, the feasible region for \eqref{eqn:max_big_m} has dimension $\eta+d$. In order to show that the constraint is facet-defining, we identify $\eta+d$ affinely independent feasible points for the MIP that satisfy the given constraint at equality.

Fix a point $\hat{x}$ in the interior of $D_{|\ell}$, which exists since $D_{|\ell}$ has dimension $\eta$. Denote the feasible point $p^0 = (\hat{x}, f^\ell(\hat{x}), {\bf e}^\ell)$. Since $\hat{x}$ is in the interior of $D_{|\ell}$, there exists a sufficiently small $\epsilon > 0$ such that the points $p^i = (\hat{x} + \epsilon {\bf e}^i, f^\ell(\hat{x} + \epsilon {\bf e}^i), {\bf e}^\ell)$ are feasible for all $i \in \llbracket \eta \rrbracket$. Note that each of the $\eta+1$ points $p^0, p^1, \ldots, p^\eta$ satisfies the constraint at equality.

Now for each $k \in \llbracket d \rrbracket \backslash \{\ell\}$, take the point $\tx^k \in \arg\max_{\tx \in D_{|k}}f^k(\tx)-f^\ell(\tx)$, along with $\tilde{p}^k = (\tx^k, f^k(\tx^k), {\bf e}^k)$. This point $\tilde{p}^k$ is feasible for \eqref{eqn:max_big_m}, and satisfies the given constraint at equality.

To finish, we must show that the $\eta + d$ points constructed thus far are affinely independent. Presume w.l.o.g. that $\ell = 1$. The result follows by showing the following matrix has full row rank:
\[
    \begin{pmatrix} \tilde{p}^2 - p^0 \\ \vdots \\ \tilde{p}^d - p^0 \\ p^1 - p^0 \\ \vdots \\ p^\eta - p^0  \end{pmatrix} = \begin{pmatrix} 
        \tx^2 - \hat{x} & f^2(\tx^2) - f^1(\hat{x}) & {\bf e}^2 - {\bf e}^1 \\
        \vdots & \vdots & \vdots \\
        \tx^d - \hat{x} & f^d(\tx^d) - f^1(\hat{x}) & {\bf e}^d - {\bf e}^1 \\
        \epsilon {\bf e}^1 & w_1 \epsilon & 0 \\
        \vdots & \vdots & \vdots \\
        \epsilon {\bf e}^\eta & w_\eta \epsilon & 0
    \end{pmatrix}.
\]
If we permute the last $d-1$ columns (corresponding to the $z_2$ to $z_d$ variables) to the first $d-1$ columns, we observe that the resulting matrix is upper triangular with a nonzero diagonal, and so has full row rank. Therefore, the starting matrix also has full row rank, as we only applied elementary row operations, and therefore the $\eta+d$ points are affinely independent, giving the result. 

\qed\end{proof}
