# Supplementary material for: Strong mixed-integer programming formulations for trained neural networks
Source: arXiv:1811.01988 source file (2020-01-21)
Supplement: Supplementary file 2 [file appendix-E.tex]

\section{Proof of Proposition~\ref{prop:unary-clipped-relu-formulation}} \label{app:clipped-relu}

We separately prove each of the three parts of Proposition~\ref{prop:unary-clipped-relu-formulation}.
\begin{customproposition}{\ref{prop:unary-clipped-relu-formulation} (Part 1)}
    Take some affine function $f(x) = w \cdot x + b$ over input domain $D = [L,U]$. The following is a valid formulation for $\gr(\emph{\Clipped{}} \circ f; [L,U])$:
    \begin{subequations} 
    \begin{align}
        C z_3 &\leq y \leq C(z_2 + z_3)  \tag{\ref{eqn:unary-clipped-relu-formulation-1}}\\
        y &\leq f(x) - M^-(f)z_1\tag{\ref{eqn:unary-clipped-relu-formulation-2}} \\
        y &\geq f(x) + \left(C-M^+(f)\right)z_3  \tag{\ref{eqn:unary-clipped-relu-formulation-3}}\\
        1 & =z_1 + z_2 + z_3   \tag{\ref{eqn:unary-clipped-relu-formulation-4}}\\
        (x,y,z) &\in [L,U] \times \bbR_{\geq 0} \times [0,1]^3  \tag{\ref{eqn:unary-clipped-relu-formulation-5}}\\
        z &\in \{0,1\}^3.  \tag{\ref{eqn:unary-clipped-relu-formulation-6}}
    \end{align}
    \end{subequations}
\end{customproposition}
\begin{proof}
If $z=(1,0,0)$, then the (\ref{eqn:unary-clipped-relu-formulation-1}-\ref{eqn:unary-clipped-relu-formulation-3},\ref{eqn:unary-clipped-relu-formulation-5}) reduces to
\[
    P^1 = \Set{(x,y) \in [L,U] \times \bbR_{\geq 0} | \begin{array}{c} y = 0 \\ f(x) \geq M^-(f) \\ y \geq f(x)
    \end{array} }.
\]
If $z=(0,1,0)$, then the (\ref{eqn:unary-clipped-relu-formulation-1}-\ref{eqn:unary-clipped-relu-formulation-3},\ref{eqn:unary-clipped-relu-formulation-5}) reduces to
\[
    P^2 = \Set{(x,y) \in [L,U] \times \bbR_{\geq 0} | \begin{array}{c} 0 \leq y \leq C \\ y \leq f(x) \\ y \geq f(x)
    \end{array} }.
\]
If $z=(0,0,1)$, then the (\ref{eqn:unary-clipped-relu-formulation-1}-\ref{eqn:unary-clipped-relu-formulation-3},\ref{eqn:unary-clipped-relu-formulation-5}) reduces to
\[
    P^3 = \Set{(x,y) \in [L,U] \times \bbR_{\geq 0} | \begin{array}{c} y = C \\ y \leq f(x) \\ f(x) \leq M^+(f)
    \end{array} }.
\]
This exhausts all feasible values for $z$ with respect to (\ref{eqn:unary-clipped-relu-formulation-4},\ref{eqn:unary-clipped-relu-formulation-6}). Furthermore, $\gr(\Clipped{} \circ f; [L,U]) = P^1 \cup P^2 \cup P^3$, giving the result.
\qed \end{proof}

\begin{customproposition}{\ref{prop:unary-clipped-relu-formulation} (Part 2)}
    Moreover, the following inequalities are valid for \eqref{eqn:unary-clipped-relu-formulation}:
    \begin{alignat}{2}
        % y &\leq \sum_{i \in I} w_ix_i - \sum_{i \in I}m_iz_1 + \left(b + \sum_{i \not\in I}N_i\right)z_2 + \min\left\{C - \sum_{i \in I}m_i, b + \sum_{i \not\in I}N_i \right\}z_3 \quad \forall I \subseteq \supp(w) \label{eqn:unary-clipped-cut-1} \\
        % y &\geq \sum_{i \in I} w_ix_i + \max\left\{ -\sum_{i \in I}N_i, b + \sum_{i \not\in I}m_i \right\}z_1 + \left(b + \sum_{i \in I}m_i\right)z_2 + \left(C - \sum_{i \in I}N_i\right)z_3 \quad \forall I \subseteq \supp(w) \label{eqn:unary-clipped-cut-2}.
        % y &\leq \sum_{i \in I} w_i(x_i - \breve{L}_iz_1) + \left( b + \sum_{i \not\in I} w_i\breve{U}_i \right) (z_2+z_3) \quad \forall I \subseteq \supp(w) \label{eqn:unary-clipped-cut-1} \\
        y &\leq \sum_{i \in I} w_ix_i + \left( b + \sum_{i \not\in I} w_i\breve{U}_i \right) (z_2+z_3) - \left(\sum_{i \in I} w_i \breve{L}_i\right) z_1 \quad &\forall I \subseteq \llbracket \eta \rrbracket \tag{\ref{eqn:unary-clipped-cut-1}} \\
        y &\geq \sum_{i \in I} w_ix_i + \left( b + \sum_{i \not\in I} w_i\breve{L}_i \right) (z_1+z_2) - \left(\sum_{i \in I} w_i\breve{U}_i - C\right)z_3 \quad &\forall I \subseteq \llbracket \eta \rrbracket . \tag{\ref{eqn:unary-clipped-cut-2}}
    \end{alignat}
    Additionally, the most violated inequality from the either \eqref{eqn:unary-clipped-cut-1} or \eqref{eqn:unary-clipped-cut-2} can be separated in $\mathcal{O}(\eta)$ time.
\end{customproposition}
\begin{proof}
Fix some subset $I \subseteq \llbracket \eta \rrbracket$.

\underline{Validity of \eqref{eqn:unary-clipped-cut-1}}.
Follows by case analysis: when $z=(1,0,0)$, the inequality reduces to
\[
    y \leq \sum_{i \in I} w_i(x_i - \breve{L}_i),
\]
whose validity follows as $w_ix_i \geq w_i\breve{L}_i$ for all $i$. If $z=(0,1,0)$ or $z=(0,0,1)$, then $y \leq w \cdot x + b$ is a valid inequality, and \eqref{eqn:unary-clipped-cut-1} reduces to
\[
    y \leq \sum_{i \in I}w_ix_i + \sum_{i \not\in I}w_i\breve{U}_i + b,
\]
whose validity follows from the bounds $w_ix_i \leq w_i\breve{U}_i$ for all $i$.

\underline{Validity of \eqref{eqn:unary-clipped-cut-2}}.
Consider the case when $z=(1,0,0)$ or $z=(0,1,0)$, in which case the inequality $y \geq w \cdot x + b$ is valid, and the inequality \eqref{eqn:unary-clipped-cut-2} reduces to
\[
    y \geq \sum_{i \in I} w_ix_i + \sum_{i \not\in I} w_i\breve{L}_i + b,
\]
whose validity then follows from the bounds $w_ix_i \geq w_i\breve{L}_i$ for all $i$. If $z=(0,0,1)$, then $y=C$ is valid, and the inequality \eqref{eqn:unary-clipped-cut-2} reduces to
\[
    y \geq C + \sum_{i \in I} w_i(x_i-\breve{U}_i),
\]
whose validity follows from the bounds $w_ix_i \leq w_i\breve{U}_i$ for all $i$.

Finally, observe that separation over both \eqref{eqn:unary-clipped-cut-1} and \eqref{eqn:unary-clipped-cut-2} can be performed by a single pass through the input components $i \in \llbracket \eta \rrbracket$, as minimizing the right-hand side of either inequality can be done in a completely separable manner.
\qed \end{proof}

\begin{customproposition}{\ref{prop:unary-clipped-relu-formulation} (Part 3)}
    Finally, take $\phi(I) \defeq \sum_{i \in I} w_i\breve{L}_i + \sum_{i \not\in I} w_i\breve{U}_i + b$. Then \eqref{eqn:unary-clipped-cut-1} is facet-defining if and only if $\phi(I) < C$, and \eqref{eqn:unary-clipped-cut-2} is facet-defining if and only if $\phi(\llbracket \eta \rrbracket \backslash I) > 0$.
    % Finally, for each point $(\hat{x},\hat{y},\hat{z})$ feasible for the LP relaxation of \eqref{eqn:unary-clipped-relu-formulation}, inequalities from at most one of the families \eqref{eqn:unary-clipped-cut-1} and \eqref{eqn:unary-clipped-cut-2} are violated.
\end{customproposition}
\begin{proof}
\underline{``Only-if'' direction}.
To show the only-if direction for \eqref{eqn:unary-clipped-cut-1}, we observe that when $\phi(I) \geq C$, we can express \eqref{eqn:unary-clipped-cut-1} as a conic combination of other constraints in the following way:

\begin{align*}
y \leq C(z_2+z_3) && \times&\quad 1 \\
w_i\breve{L}_i \leq w_ix_i && \times&\quad 1 & \forall i \in I \\
0 \leq z_2 && \times&\quad \phi(I) - C \\
0 \leq z_3 && \times&\quad \phi(I) - C,
\end{align*}
and then simplifying using the equation $z_1 + z_2 + z_3 = 1$.

To show the only-if direction for \eqref{eqn:unary-clipped-cut-2}, we observe that when $\phi(\llbracket \eta \rrbracket \backslash I) \leq 0$, we can express \eqref{eqn:unary-clipped-cut-2} as a conic combination of the other constraints in the following way:

\begin{align*}
y \geq Cz_3 && \times&\quad 1 \\
w_i\breve{U}_i \geq w_ix_i && \times&\quad 1 & \forall i \in I \\
z_1 \geq 0 && \times&\quad -\phi(\llbracket \eta \rrbracket \setminus I) \\
z_2 \geq 0 && \times&\quad -\phi(\llbracket \eta \rrbracket \setminus I),
\end{align*}
and then simplifying using the equation $z_1 + z_2 + z_3 = 1$.

\underline{``If'' direction}.
To show that each inequality in the family \eqref{eqn:unary-clipped-cut-1} with $\phi(I) < C$ (resp. \eqref{eqn:unary-clipped-cut-2} with $\phi(\llbracket \eta \rrbracket \setminus I) > 0$) is facet-defining under the strict activity assumption, presume w.l.o.g. that $w \geq 0$; if this is not the case, in the argument below replace $L$ and $U$ with $\breve{L}$ and $\breve{U}$, respectively, and take care to either add or subtract $\epsilon$ perturbations appropriately to maintain feasibility. Take the points $p^1 = (x,y,z) = (L,0,{\bf e}^1)$ and $p^3 = (x,y,z) = (U,C,{\bf e}^3)$, which are both feasible for \eqref{eqn:unary-clipped-relu-formulation} under our assumptions, and satisfy any inequality \eqref{eqn:unary-clipped-cut-1} or \eqref{eqn:unary-clipped-cut-2} at equality. Take some sufficiently small $\epsilon > 0$, and define the points $p^{1,i} = (L + \epsilon {\bf e}^i, 0, {\bf e}^1)$ for each $i \notin I$. By strict activity, such an $\epsilon$ exists such that each point is feasible for \eqref{eqn:unary-clipped-relu-formulation}, and satisfies the inequalities in \eqref{eqn:unary-clipped-cut-1} and \eqref{eqn:unary-clipped-cut-2} corresponding to $I$ at equality.

Take some $\mathring{x} \in [L,U]$ where: $0 < w \cdot \mathring{x} + b < C$, $\mathring{x}_i = U_i$ (resp. $\mathring{x}_i = L_i$) for each $i \not\in I$, and $L_i < \mathring{x}_i < U_i$ for each $i \in I$. For example, in the case of \eqref{eqn:unary-clipped-cut-1}, the point $\mathring{x}$ exists as it can be found as a convex combination between the point $U$ (where $f(U) > C$ by strict activity and $w \geq 0$) and the point $\tilde{x}$ given by $\tilde{x}_i = L_i$ for $i \in I$ and $\tilde{x}_i = U_i$ for $i \notin I$, for which $f(\tilde{x}) = \phi(I) < C$. The analogous is true for \eqref{eqn:unary-clipped-cut-2} with $\phi(\llbracket \eta \rrbracket \setminus I) > 0$. Take the points $p^2 = (\mathring{x},f(\mathring{x}),{\bf e}^2)$ and $p^{2,k} = (\mathring{x}+\delta {\bf e}^k, f(\mathring{x}) + w_k\delta, {\bf e}^2)$ for each $k \in I$. For sufficiently small $\delta$, each point is feasible for \eqref{eqn:unary-clipped-relu-formulation}, and satisfies the inequalities in \eqref{eqn:unary-clipped-cut-1} and \eqref{eqn:unary-clipped-cut-2} corresponding to $I$ at equality.

% By the assumptions on strict activity and that $\phi(I) < C$ (resp. $\phi(\llbracket \eta \rrbracket \setminus I) > 0$), such a point exists.

% To finish, we must show that the $\eta + 3$ points constructed thus far are affinely independent. To show this, it suffices to show that the matrix with rows $p^{1,k}-p^1$ for $k \not\in I$, $p^2-p^1$, $p^{2,k}-p^1$ for $k \in I$, and $p^3-p^1$ has full row rank. This follows after subtracting the $p^2-p^1$ row from rows $p^{2,k}-p^1$, then subtracting each row $p^{1,k}-p^1$ and $p^{2,\ell}-p^2$ (appropriately scaled by $-\frac{\mathring{x}_k-L_k}{\epsilon}$ and $-\frac{\mathring{x}_\ell-L_\ell}{\delta}$, respectively) from rows $p^2-p^1$, then subtracting them (again suitably rescaled) from row $p^3-p^1$, and rearranging the rows and columns. 

% {\color{red} Below is adapted from above:}
To finish, we must show that the $\eta + 3$ points constructed thus far are affinely independent. Presume w.l.o.g. that $I = \llbracket \kappa \rrbracket$ for some $\kappa \in \llbracket \eta \rrbracket$.
\[
    \begin{pmatrix} p^2 - p^1 \\ p^3 - p^1 \\ p^{2,1} - p^1 \\ \vdots \\ p^{2,\kappa} - p^1 \\ p^{1,\kappa+1} - p^1 \\ \vdots \\ p^{1,\eta} - p^1 \end{pmatrix} = \begin{pmatrix} 
        \mathring{x} - L &  f(\mathring{x}) - f(L) & {\bf e}^2 - {\bf e}^1 \\
        \mathring{x} - U &  f(\mathring{x}) - f(U) & {\bf e}^2 - {\bf e}^3 \\
        \mathring{x} - L + \delta {\bf e}^1 & f(\mathring{x}) - f(L) + w_1 \delta & {\bf e}^2 - {\bf e}^1 \\
        \vdots & \vdots & \vdots \\
        \mathring{x} - L + \delta {\bf e}^\kappa & f(\mathring{x}) - f(L) + w_\kappa \delta & {\bf e}^2 - {\bf e}^1 \\
        \epsilon {\bf e}^{\kappa+1} & w_{\kappa+1} \epsilon & 0 \\
        \vdots & \vdots & \vdots \\
        \epsilon {\bf e}^{\eta} & w_{\eta} \epsilon & 0 \\
    \end{pmatrix}.
\]
Now subtract the $p^2-p^1$ row from rows $p^{2,k} - p^1$ to yield
\[
    \begin{pmatrix} 
        \mathring{x} - L &  f(\mathring{x}) - f(L) & {\bf e}^2 - {\bf e}^1 \\
        \mathring{x} - U &  f(\mathring{x}) - f(U) & {\bf e}^2 - {\bf e}^3 \\
        \delta {\bf e}^1 & w_1 \delta & 0 \\
        \vdots & \vdots & \vdots \\
        \delta {\bf e}^\kappa & w_\kappa \delta & 0 \\
        \epsilon {\bf e}^{\kappa+1} & w_{\kappa+1} \epsilon & 0 \\
        \vdots & \vdots & \vdots \\
        \epsilon {\bf e}^{\eta} & w_{\eta} \epsilon & 0 \\
    \end{pmatrix}.
\]
If we permute the last three columns (corresponding to the $z$ variables) to the first three columns, we observe that the resulting matrix is upper triangular with a nonzero diagonal, and so has full row rank. Therefore, the starting matrix also has full row rank, as we only applied elementary row operations, and therefore the $\eta+3$ points are affinely independent, giving the result. 
\qed \end{proof}
